# Supplementary material for: A rich population of free-floating planets in the Upper Scorpius young stellar association
Source: arXiv:2112.11999 source file (2021-12-22)
Supplement: Supplementary file 1 [file Supplement.pdf]

## Supplementary Information

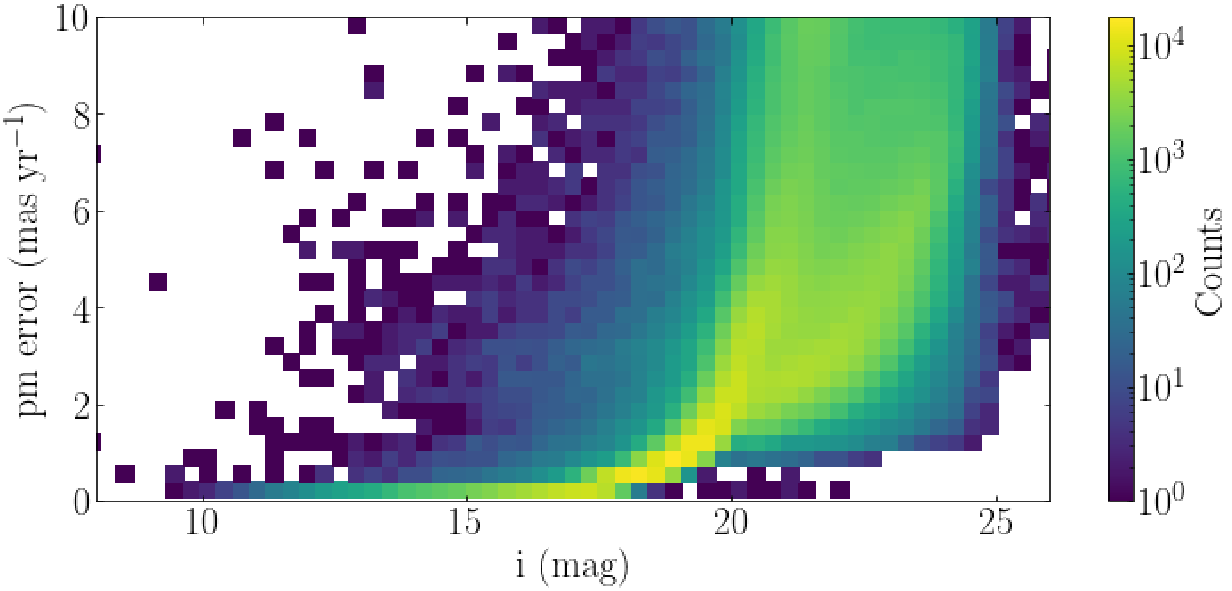


Supplementary Figure 1: Estimated proper motion error as a function of $i$ magnitude for the DANCe catalogue. We note that whenever there is a proper motion measure from *Gaia* we use it. This explains the change in precision observed at $i \sim 21$ mag.

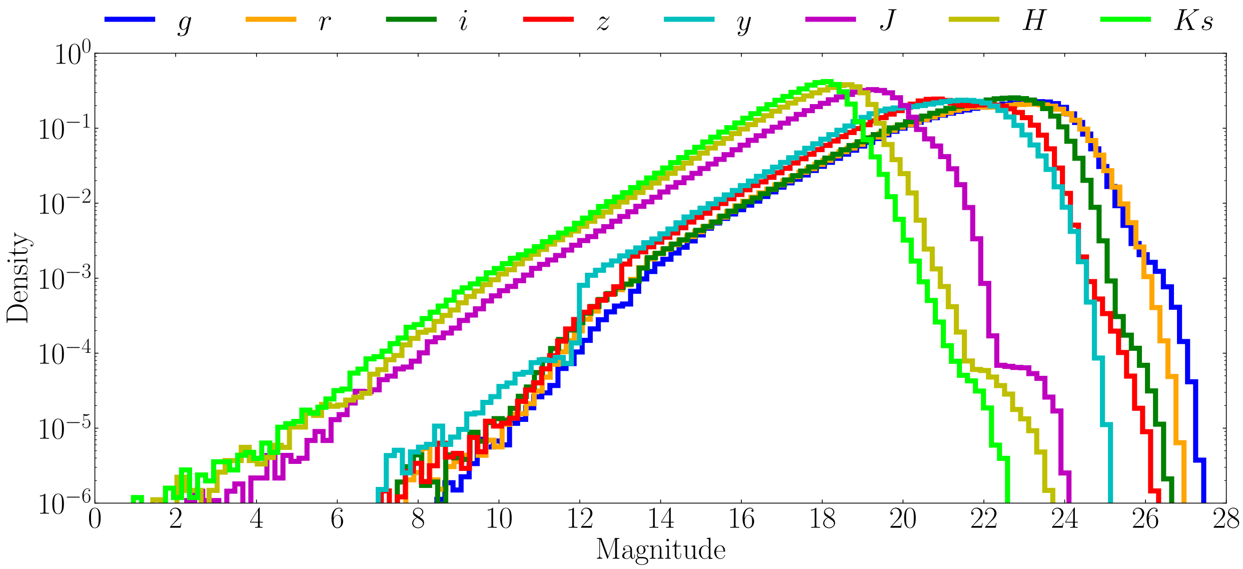


Supplementary Figure 2: Density of sources per 0.2 magnitude bin as a function of magnitude for all the sources in the DANCe catalogue.

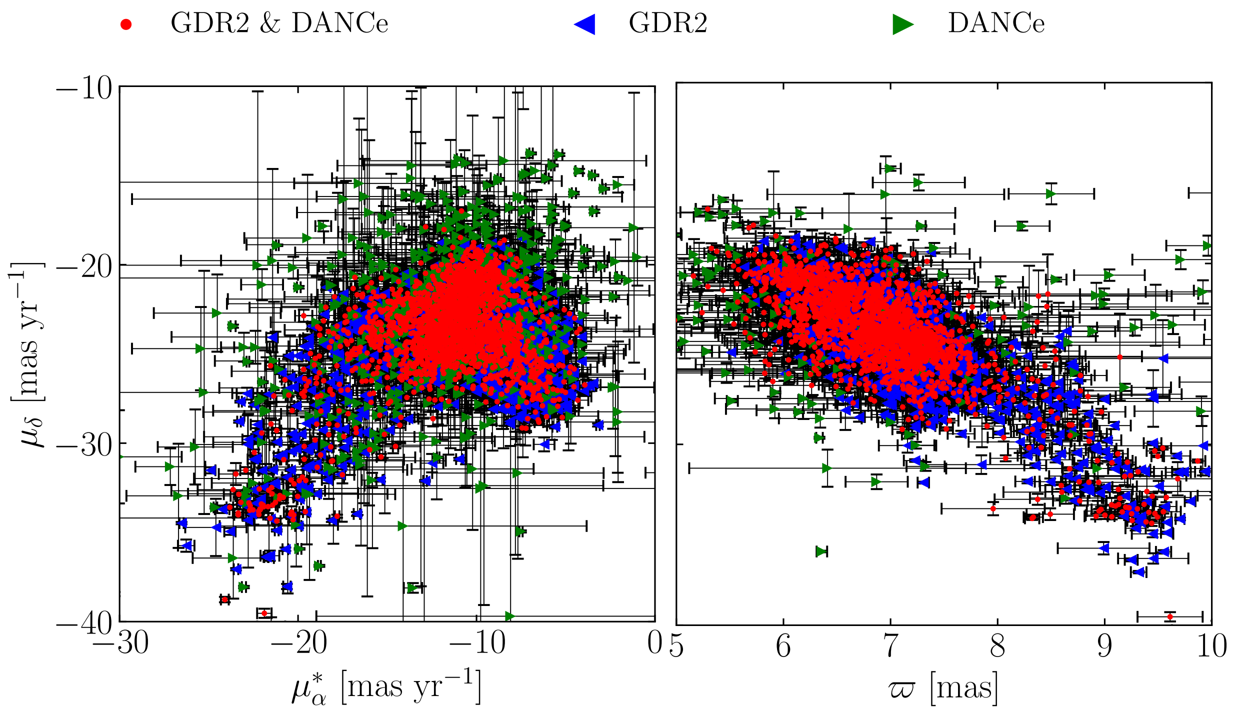


Supplementary Figure 3: Vector point diagram (left) and parallax–proper motion diagram (right) of USC and Oph. The members are shape- and colour-coded according their origin: *Gaia* and DANCe analysis (red circles), only *Gaia* analysis (blue left-pointing triangle), and only DANCe analysis (green right-pointing triangle). The error bars represent the astrometric uncertainties reported in the *Gaia* and DANCe catalogues.

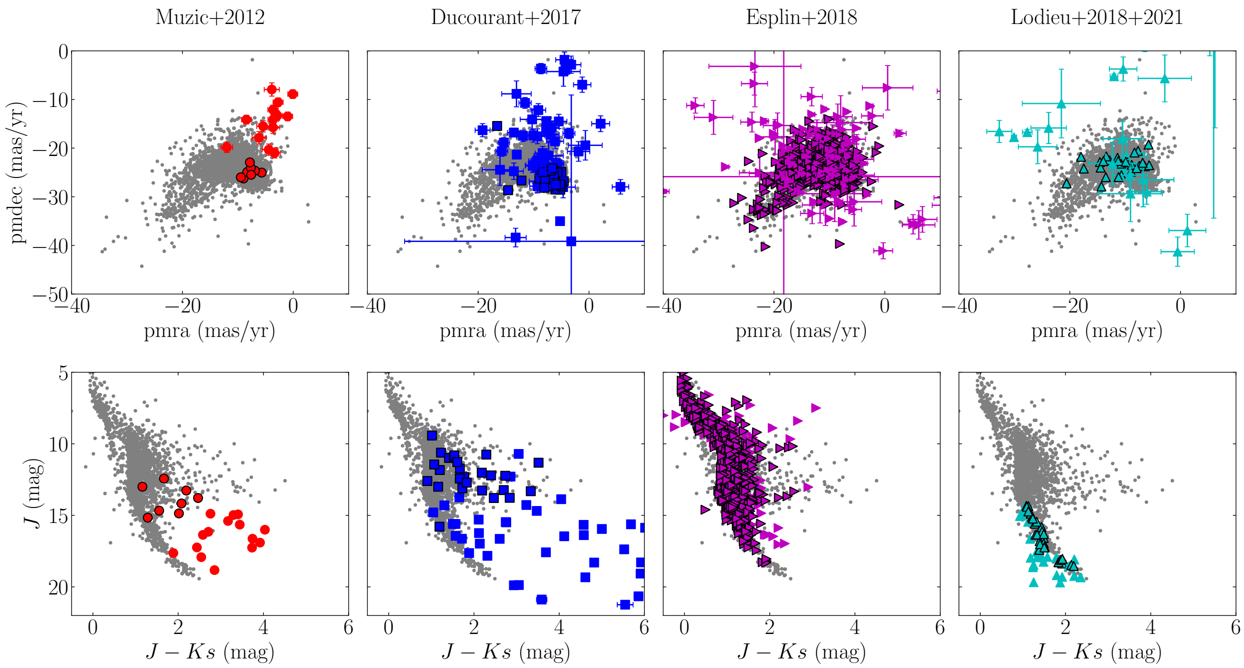


Supplementary Figure 4: Vector point diagrams (top) and colour-magnitude diagrams (bottom) of the members found in this study (grey dots) and the members reported in previous studies[1–5] (coloured markers). The members in common are indicated by a black edge line. The error bars represent the observational uncertainties in the *Gaia* and DANCe catalogues for the members previously identified in the literature and discarded by our membership analysis. We note that our study is not sensitive to highly extinct areas or the detection of sources with moderate/significant near-infrared excess.

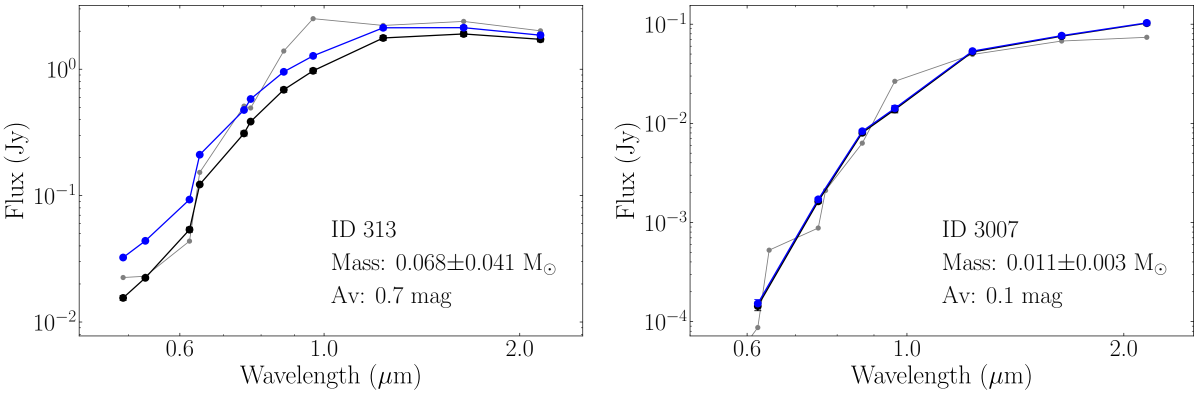


Supplementary Figure 5: Spectral energy distribution of two of our substellar objects: a brown dwarf mass object (left) and a planetary-mass object (right). The photometric observations (black) and the dereddened observations (blue) are indicated. The error bars represent the photometric uncertainties and are smaller than the markers in most cases. The BHAC15 models at 5 Myr used for the best-fit models are shown (gray).

Supplementary Table 1: Instruments used in the DANCe catalogue of USC and Oph.

| Telescope | Instrument | Filters | Platescale [pixel$^{-1}$] | Field of view | Epoch Min./Max. | Images |
|---|---|---|---|---|---|---|
| ESO VISTA[6] | VIRCAM | $z, J, H, K$ | $0\farcs34$ | $1.2^\circ \times 1.1^\circ$ | 2010–2018 | 18 598 |
| ESO VST[7] | OmegaCAM | $u, g, r, i, z, H\alpha$ | $0\farcs21$ | $1^\circ \times 1^\circ$ | 2014–2017 | 3 302 |
| ESO VLT[8] | VIMOS | $R, I, Z$ | $0\farcs205$ | $28' \times 32'$ | 2007-2011 | 261 |
| ESO VLT[9] | HAWK-I | $y, J, H, K$ [a] | $0\farcs106$ | $7.5' \times 7.5'$ | 2008–2015 | 2 752 |
| ESO (2.2 m)[10] | WFI | $B, V, R, I$ [a] | $0\farcs24$ | $34' \times 33'$ | 2000–2017 | 1 562 |
| CTIO (Blanco)[11] | DECam | $u, g, r, i, z, y$ [a] | $0\farcs27$ | $1.1^\circ$ radius | 2012–2018 | 3 744 |
| CTIO (Blanco)[12] | ISPI | $J, H, K$ [a] | $0\farcs3$ | $10.25' \times 10.25'$ | 2005–2010 | 2 214 |
| CTIO (Blanco)[13] | NEWFIRM | $J, H, K$ [a] | $0\farcs4$ | $28' \times 28'$ | 2010–2011 | 1 348 |
| KPNO (Mayall)[13] | NEWFIRM | $J, H, K$ [a] | $0\farcs4$ | $28' \times 28'$ | 2013–2014 | 247 |
| CFHT[14] | MegaCam | $u, g, r, i$ [a] | $0\farcs18$ | $1^\circ \times 1^\circ$ | 2004–2016 | 1 395 |
| CFHT[15] | WIRCam | $y, J, H, K$ [a] | $0\farcs3$ | $20' \times 20'$ | 2007–2017 | 6 579 |
| CFHT[16] | CFH12K | $B, V, r, i, z$ | $0\farcs21$ | $42' \times 28'$ | 2000–2002 | 438 |
| INT[17] | WFC | $B, V, R, I, Z, g, r, i$ [a] | $0\farcs33$ | $34' \times 34'$ | 2000–2014 | 430 |
| UKIRT[18] | WFCAM | $z, y, J, H, K$ [a] | $0\farcs4$ | $40' \times 40'$ [b] | 2005-2012 | 34 837 |
| SDSS[19] | SDSS Imaging Camera | $u, g, r, i, z$ | $0\farcs396$ | | 2005–2009 | 2 112 |
| Subaru[20] | HSC | $r, i, Y$ | $0\farcs17$ | $1.8^\circ$ radius | 2015–2017 | 160 |
| Subaru[21] | Suprime-Cam | $g, r, i, z, V, R, I$ [a] | $0\farcs2$ | $34' \times 27'$ | 2004–2011 | 804 |
| Palomar 48" [22] | PTF | $g, r$ | $1\farcs0$ | $3\fdg3 \times 2\fdg2$ [c] | 2010–2014 | 35 |

[a]as well as narrow and medium bands

[b]the chip layout has large gaps between detectors, and the coverage of the focal plane is only partial

[c]one of the 12 detectors is dead

1. Mužić, K., Scholz, A., Geers, V., Jayawardhana, R. & Tamura, M. Substellar Objects in Nearby Young Clusters (SONYC). V. New Brown Dwarfs in $\rho$ Ophiuchi. *Astrophys. J.* **744**, 134 (2012).

2. Ducourant, C. *et al.* Proper motion survey and kinematic analysis of the $\rho$ Ophiuchi embedded cluster. *Astron. Astrophys.* **597**, A90 (2017).

3. Esplin, T. L., Luhman, K. L., Miller, E. B. & Mamajek, E. E. A WISE Survey of Circumstellar Disks in the Upper Scorpius Association. *Astron. J.* **156**, 75 (2018).

4. Lodieu, N., Zapatero Osorio, M. R., Béjar, V. J. S. & Peña Ramírez, K. The optical + infrared L dwarf spectral sequence of young planetary-mass objects in the Upper Scorpius association. *Mon. Not. R. Astron. Soc.* **473**, 2020–2059 (2018).

5. Lodieu, N., Hambly, N. C. & Cross, N. J. G. Exploring the planetary-mass population in the Upper Scorpius association. *Mon. Not. R. Astron. Soc.* **503**, 2265–2279 (2021).

6. Emerson, J., McPherson, A. & Sutherland, W. Visible and Infrared Survey Telescope for Astronomy: Progress Report. *The Messenger* **126**, 41–42 (2006).

7. Kuijken, K. *et al.* OmegaCAM: the 16k×16k CCD camera for the VLT survey telescope. *The Messenger* **110**, 15–18 (2002).

8. Le Fèvre, O. *et al.* Commissioning and performances of the VLT-VIMOS instrument. In Iye, M. & Moorwood, A. F. M. (eds.) *Instrument Design and Performance for Optical/Infrared Ground-based Telescopes*, vol. 4841 of *Society of Photo-Optical Instrumentation Engineers (SPIE) Conference Series*, 1670–1681 (2003).

9. Pirard, J.-F. *et al.* HAWK-I: A new wide-field 1- to 2.5-$\mu$m imager for the VLT. In Moorwood, A. F. M. & Iye, M. (eds.) *Ground-based Instrumentation for Astronomy*, vol. 5492 of *Society of Photo-Optical Instrumentation Engineers (SPIE) Conference Series*, 1763–1772 (2004).

10. Baade, D. *et al.* The Wide Field Imager at the 2.2-m MPG/ESO telescope: first views with a 67-million-facette eye. *The Messenger* **95**, 15–16 (1999).

11. Flaugher, B. L. *et al.* Status of the dark energy survey camera (DECam) project. In *Ground-based and Airborne Instrumentation for Astronomy III*, vol. 7735 of *Proc. SPIE*, 77350D (2010).

12. van der Bliek, N. S. *et al.* ISPI: a wide-field NIR imager for the CTIO Blanco 4-m telescope. In Moorwood, A. F. M. & Iye, M. (eds.) *Ground-based Instrumentation for Astronomy*, vol. 5492 of *Society of Photo-Optical Instrumentation Engineers (SPIE) Conference Series*, 1582–1589 (2004).

13. Autry, R. G. *et al.* NEWFIRM: the widefield IR imager for NOAO 4-m telescopes. In M. Iye & A. F. M. Moorwood (ed.) *Society of Photo-Optical Instrumentation Engineers (SPIE) Conference Series*, vol. 4841 of *Society of Photo-Optical Instrumentation Engineers (SPIE) Conference Series*, 525–539 (2003).

14. Boulade, O. *et al.* MegaCam: the new Canada-France-Hawaii Telescope wide-field imaging camera. In M. Iye & A. F. M. Moorwood (ed.) *Society of Photo-Optical Instrumentation Engineers (SPIE) Conference Series*, vol. 4841 of *Society of Photo-Optical Instrumentation Engineers (SPIE) Conference Series*, 72–81 (2003).

15. Thibault, S., Lacoursiere, J., Artigau, E., Vallee, P. & Doyon, R. Optical design of CPAPIR, a cryogenic IR camera for OMM. In *International Optical Design Conference 2002*, vol. 4832 (2002).

16. Cuillandre, J.-C., Luppino, G. A., Starr, B. M. & Isani, S. Performance of the CFH12K: a 12K by 8K CCD mosaic camera for the CFHT prime focus. In Iye, M. & Moorwood, A. F. (eds.) *Society of Photo-Optical Instrumentation Engineers (SPIE) Conference Series*, vol. 4008 of *Presented at the Society of Photo-Optical Instrumentation Engineers (SPIE) Conference*, 1010–1021 (2000).

17. Ives, D. The INT Wide Field Camera. *IEEE Spectrum* **16**, 20–21 (1998).

18. Casali, M. *et al.* The UKIRT wide-field camera. *Astron. Astrophys.* **467**, 777–784 (2007).

19. Alam, S. *et al.* The Eleventh and Twelfth Data Releases of the Sloan Digital Sky Survey: Final Data from SDSS-III. *Astrophys. J. Suppl. Ser.* **219**, 12 (2015).

20. Miyazaki, S. *et al.* Hyper Suprime-Cam: System design and verification of image quality. *Publ. Astron. Soc. Jpn* **70**, S1 (2018).

21. Miyazaki, S. *et al.* Subaru Prime Focus Camera – Suprime-Cam. *Publ. Astron. Soc. Jpn* **54**, 833–853 (2002).

22. Rahmer, G. *et al.* *The 12K×8K CCD mosaic camera for the Palomar Transient Factory*, vol. 7014 of *Society of Photo-Optical Instrumentation Engineers (SPIE) Conference Series*, 70144Y (2008).

Supplementary Table 2: Performance of the membership analysis.

| | *Hipparcos* | | | | *Gaia* | | | | DANCe | | | |
|---|---|---|---|---|---|---|---|---|---|---|---|---|
| $p_{in}$ | $p_{opt}$ | Memb | CR (%) | TPR (%) | $p_{opt}$ | Memb | CR (%) | TPR (%) | $p_{opt}$ | Memb | CR (%) | TPR (%) |
| 0.5 | 0.97 | 116 | 17 | 92 | 0.95 | 2 762 | 1.1 | 99.2 | 0.77 | 2 556 | 2 | 98 |
| 0.6 | 0.96 | 108 | 7 | 95 | 0.96 | 2 698 | 0.9 | 99.2 | 0.78 | 2 458 | 2 | 99 |
| 0.7 | 0.94 | 112 | 7 | 96 | 0.96 | 2 678 | 1.0 | 99.4 | 0.83 | 2 342 | 1.5 | 99 |
| 0.8 | 0.95 | 103 | 5 | 96 | 0.96 | 2 661 | 0.9 | 99.6 | 0.88 | 2 185 | 0.9 | 99 |
| 0.9 | 0.96 | 78 | 3 | 98 | 0.96 | 2 623 | 0.9 | 99.6 | 0.83 | 2 086 | 0.9 | 99 |

Performance of the membership analysis obtained with different internal probability thresholds ($p_{in}$) for the three catalogues considered, namely *Hipparcos*, *Gaia*, and DANCe. For each internal probability threshold ($p_{in}$) we show the corresponding optimum probability threshold ($p_{opt}$), number of members (Memb), contamination rate (CR) and true positive rate (TPR). The $p_{opt}$, CR, and TPR were obtained with synthetic data (see text).
